# Supplementary material for: Incentivizing Combinatorial Bandit Exploration
Source: arXiv:2206.00494 source file (2022-06-01)
Supplement: Supplementary file 1 [file app-errata-neurips22subm.tex]

\section{\textbf{ERRATA} for the body of the paper}

We've noticed some minor issues in \Cref{subsec:cyclic} that do not substantially change the results. Recall that \Cref{subsec:cyclic} is on initial exploration by reduction to incentivized exploration for $K$-armed bandits.

First, \Cref{thm-P2-gen-typo}, the result for an arbitrary set of feasible arms, should have a different definition of $\tau_\calP$, with a corresponding change in \Cref{cor-p2-gen-typo}; see \Cref{subsec:initial-general} for the correct statements. The results remain qualitatively similar. Note that the results for the special case (when the arms are all subsets of $m$ atoms, \Cref{thm-P2-beta} and \Cref{cor-p2-beta}) remain unaffected.

Second, $\kappa(n)$, the number of arms in the sequence of arms defined in \Cref{subsec:cyclic}, could be infinite for some $n\in\N$. The sequence stops when the arms therein cover all atoms at least once (as we wrote in the body), and continues indefinitely otherwise. In \Cref{thm-P2-beta} and \Cref{thm-P2-gen-typo}, we prove that the sequence length $\kappa = \kappa(\myNp)$ is finite and upper-bounded.

Also, some typos: 
\begin{OneLiners}
\item Property \PropHE should be stated with $\geq$ in \eqref{eq:P2}, instead of $>$.
\item In Line 291, the reference to Assumption (7) should be to Assumption (11).
\end{OneLiners}
